# Supplementary material for: Time-reversal symmetry breaking in the chemosensory array reveals mechanisms for dissipation-enhanced cooperative sensing
Source: arXiv:2312.17424 ancillary file (2024-07-08)
Supplement: Supplementary file 1 [file si.pdf]

# Supplemental Information: Time-reversal symmetry breaking in the chemosensory array reveals mechanisms for dissipation-enhanced cooperative sensing

David Hathcock,[1,*] Qiwei Yu,[1,2,*] and Yuhai Tu[1]

[1]IBM T. J. Watson Research Center, Yorktown Heights, NY 10598

[2]Lewis-Sigler Institute for Integrative Genomics, Princeton University, Princeton, NJ 08544

## CONTENTS

I. Supplemental analytical results S1
A. Mean-field model S1
1. Critical coupling $J_c$ in the continuum limit S2
2. Phase boundary $J_{th}(\Delta E_B)$ and superstable critical thresholds $J_{c\pm}$ S3
3. Exact solution for $k_3 \gg 1$ S4
4. Susceptibility scaling for $k_3 \gg 1$ S5
B. Effective Hill coefficient with respect to ligand concentration S7

II. Supplemental numerical results S7
A. Numerical scheme for determining the dwell time and switching time S7
B. Two-state switching in other lattice structures S8
C. Scaling of asymmetric switching statistics with lattice size S8
D. Finite-size scaling of asymmetric switching statistics in the mean-field model S9
E. Response functions S11

References S14

## I. SUPPLEMENTAL ANALYTICAL RESULTS

### A. Mean-field model

In the mean-field limit, all the sites (core units) can be treated as fully connected. The effective field experienced by site $i$ is $h_i = \frac{J}{N-1}\sum_{j\neq i} a_j = \frac{J}{N-1}(N\langle a\rangle - a_i)$. The system occupies a two-dimensional state space spanned by $(N_{-1}, N_1)$, which are the number of inactive and active sites, respectively. The kinase reactions map to a continuous-time Markov chain in this state space, with the following transitions:

$$
\begin{aligned}
(N_1, N_{-1}) &\underset{(N_1+1)k_{-1}}{\overset{N_{-1}k_1\exp\left(\frac{J(N_1-N_{-1}+1)}{N-1}\right)}{\rightleftharpoons}} (N_1+1, N_{-1}-1),\\
(N_1, N_{-1}) &\underset{(N_1+1)k_{2}}{\overset{N_{0}k_{-2}\exp\left(\frac{J(N_1-N_{-1})}{2(N-1)}\right)}{\rightleftharpoons}} (N_1+1, N_{-1}),\\
(N_1, N_{-1}) &\underset{(N_{-1}+1)k_{-3}\exp\left(\frac{J(N_1-N_{-1})}{2(N-1)}\right)}{\overset{N_0 k_3}{\rightleftharpoons}} (N_1, N_{-1}+1),
\end{aligned}
\tag{S1}
$$

where $N_0 = N - N_1 - N_{-1}$ is the number of kinases not bound to CheY or CheY-P. The steady-state probability distribution can be determined by solving the master equation:

$$
\frac{\mathrm{d}P(N_1,N_{-1},t)}{\mathrm{d}t} = \sum_{N_1',N_{-1}'}\left[P(N_1',N_{-1}',t)W[(N_1',N_{-1}')\to(N_1,N_{-1})] - P(N_1,N_{-1},t)W[(N_1,N_{-1})\to(N_1',N_{-1}')]\right] = 0,
\tag{S2}
$$

---

* These two authors contributed equally to this work.

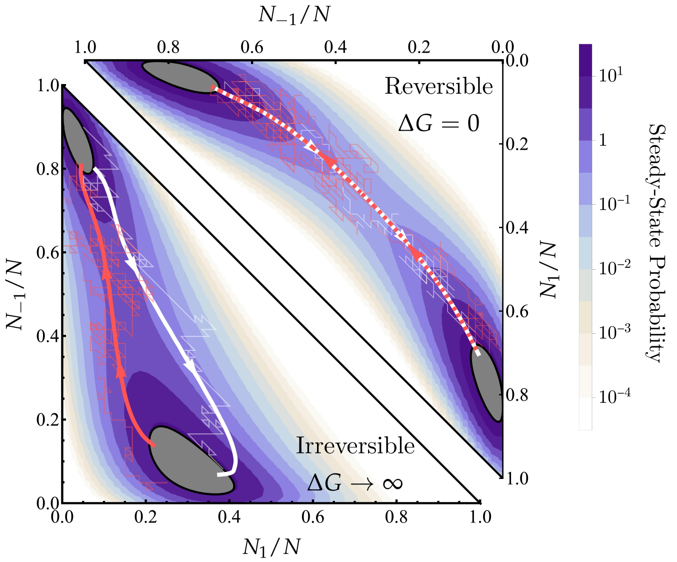


FIG. S1. Switching paths in the mean-field limit. Average forward (white) and backward (red) switching trajectories in the $(N_1, N_{-1})$–plane obtained from simulations of the mean-field model. The lower triangle shows the irreversible limit ($\Delta G \to \infty$) with asymmetric switching paths, and the upper triangle shows the reversible limit ($\Delta G = 0$) with symmetric paths. The background contours show the steady-state probability distribution. The active and inactive states are defined as those with at least 1/2 the probability of the local peaks (gray contours). Thin lines show example switching trajectories. Transition paths are nearly identical to those from the lattice model (see main text Fig. 3).

with $W[(N_1', N_{-1}') \to (N_1, N_{-1})]$ being the transition rates given in Eq. S1.

When the coupling is sufficiently strong ($J > J_c$), the steady-state probability distribution has two maxima that represent the active and inactive collective states (Fig. S1, background contours). The mean transition paths between these two states can be obtained by simulating the discrete model (Eq. S1) with the Gillespie algorithm [1]. The forward and backward transition paths (Fig. S1, white and red trajectories) are qualitatively identical to those from the lattice model, projected onto the $(N_1, N_{-1})$ state space (c.f. main text Fig. 3).

### 1. *Critical coupling $J_c$ in the continuum limit*

In the continuum limit $N \gg 1$, we introduce $x = \frac{N_1}{N}$, $y = \frac{N_{-1}}{N}$ to denote the fraction of sites in $\pm 1$ states respectively. The effective free energy landscape is defined by $F(x, y) \equiv -\ln P(x, y)$, where $P(x, y)$ is the steady state distribution for the master equation, Eq. (S2). At a sufficiently large coupling ($J > J_c$), two-state switching takes place between two local minima (i.e. metastable states) on the free energy landscape. The critical point $J = J_c$ is defined by a pitchfork bifurcation, where both minima and a saddle point coincide.

The continuum limit of the transition rates (Eq. S1) leads to the following effective force

$$f_x = k_1 y e^{J(x-y)} + k_{-2}(1 - x - y)e^{J(x-y)/2} - (k_{-1} + k_2)x, \tag{S3}$$

$$f_y = k_3(1 - x - y) + k_{-1}x - \left(k_1 e^{J(x-y)} + k_{-3} e^{J(x-y)/2}\right) y. \tag{S4}$$

The local minima of the free energy landscape are fixed points of the effective force $f_x = f_y = 0$ since the diffusion coefficients vanish as $O(N^{-1})$ in the continuum limit. To compute these fixed points, we introduce $u = x - y$ and eliminating $x$ and $y$ by solving $f_y = 0$:

$$f_y = 0 \Leftrightarrow y(u) = \frac{k_3(1-u) + \epsilon k_1 u}{k_1 e^{Ju} + \epsilon k_3 e^{Ju/2} + 2k_3 - \epsilon k_1}, \quad x(u) = y(u) + u, \tag{S5}$$

where we have introduced the reverse reaction rate scaling with dissipation, $k_{-i} = k_i e^{-\Delta G/3} \equiv k_i \epsilon$ as in the main text. Substituting $x(u)$ and $y(u)$ into $f_x = 0$ reduces the fixed point condition to a single equation, $f_u = 0$. The

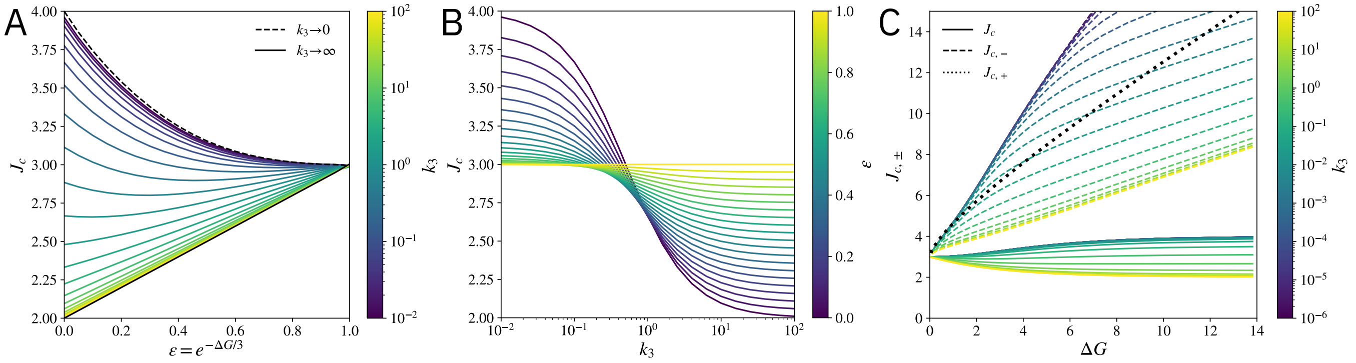


FIG. S2. (A–B) Illustration of the critical coupling $J_c$ determined from the pitchfork bifurcation condition (Eq. S6) as a function of $k_3$ and $\epsilon \equiv e^{-\Delta G/3}$. The black dashed and solid lines show limits of $k_3 \to 0$ and $k_3 \to \infty$, respectively. (C) $J_c$ (solid lines) and the critical coupling for super stable states $J_{c,-}$ (dashed lines) and $J_{c,+}$ (dotted line) as functions of $\Delta G$ for different $k_3$. Both $J_c$ and $J_{c,-}$ decrease with $k_3$, while $J_{c,+}$ is independent $k_3$. The switchable region $J \in (J_c, \min(J_{c,\pm}))$ expands with dissipation $\Delta G$.

critical coupling $J_c$ is obtained from the pitchfork bifurcation condition:

$$f_u = 0, \quad \frac{\mathrm{d}f_u}{\mathrm{d}u} = 0, \quad \frac{\mathrm{d}^2 f_u}{\mathrm{d}u^2} = 0. \tag{S6}$$

In general, this is a set of nonlinear equations that can only be solved numerically. However, we obtain analytical solutions in two special limits:

- Near-equilibrium limit ($\epsilon = 1 - \delta\epsilon$). In equilibrium ($\delta\epsilon = 0$), the bifurcation takes place at $u = 0$ with critical coupling $J_c = 3$, independent of the kinetic rates $k_i$. Indeed, since the system obeys detailed balance, the steady-state properties only depend on the ratio of forward and backward rates $k_i/k_{-i} = \epsilon^{-1} = 1$. Scaling both forward and backward rates simultaneously has no effect on the critical point. For small dissipation, to leading order in $\delta\epsilon$, we find

$$J_c = 3 - \frac{k_3}{1+k_3}\delta\epsilon, \quad k_1 = \frac{2k_3}{1+k_3} - \frac{(k_3-1)k_3}{(k_3+1)^2}\delta\epsilon, \quad u = -\frac{2}{27}\frac{3+7k_3}{(1+k_3)^2}\delta\epsilon. \tag{S7}$$

- Near-irreversible limit ($\epsilon \ll 1$). Here, the bifurcation point is:

$$J_c = \frac{4(k_2+k_3)}{k_2+2k_3} - \frac{8k_2^2 - 2k_2k_3 - 4k_3^2}{e^{\frac{k_2}{k_2+2k_3}}(k_2+2k_3)^2}\epsilon + O(\epsilon^2), \quad k_1 = \frac{k_2k_3}{k_2+k_3}e^{\frac{2k_2}{k_2+2k_3}} + O(\epsilon), \quad u = -\frac{k_2}{2(k_2+k_3)} + O(\epsilon), \tag{S8}$$

  where we have omitted the complicated linear order coefficients for $k_1$ and $u$. In the fully irreversible case ($\epsilon = 0$), the critical coupling $J_c$ decreases monotonically with the ratio $k_3/k_2$, ranging from $J_c = 4$ when $k_3/k_2 \to 0$ to $J_c = 2$ when $k_3/k_2 \to \infty$.

Fig. S2A-B shows the numerically computed critical coupling $J_c$ (from the pitchfork bifurcation condition, Eq. S6) over the full range of dissipation strength $\epsilon$ and rate $k_3$. These curves interpolate between the equilibrium and irreversible limits given above. As in the irreversible limit, $J_c$ is always monotonically decreasing with $k_3$. In the large $k_3$ limit, $J_c$ increases monotonically with $\epsilon$ (thereby decreases monotonically with $\Delta G$). Conversely, when $k_3$ is small enough, $J_c$ is non-monotonic with dissipation. In particular, $J_c(\epsilon)$ becomes non-monotonic when the $O(\epsilon)$ coefficient on $J_c(\epsilon)$ in Eq. (S8) is negative, or $k_3 < \frac{1}{4}(\sqrt{33} - 1)k_2$.

### 2. *Phase boundary $J_{th}(\Delta E_B)$ and superstable critical thresholds $J_{c\pm}$*

For a general barrier shift $\Delta E_B \neq 0$, the phase boundary is defined by a saddle-node bifurcation ($f_u = \frac{\mathrm{d}f_u}{\mathrm{d}u} = 0$), where one of the stable states (active or inactive) collides with and annihilates the barrier state. For each dissipation

level, $\Delta G$, we numerically solve this system of equations to determine the phase boundaries $J_{th}(\Delta E_B)$ shown in Fig. 5C of the main text.

The active and inactive states become superstable when the coupling is strong enough that the states cannot be removed even by arbitrarily large barrier shifts $\Delta E_B \to \pm\infty$ (corresponding to very large or small ligand concentrations). Thus, we again look for a saddle-node bifurcation in the limits of $k_1 \to 0$ and $k_1 \to +\infty$ to determine the critical thresholds $J_{c+}$ (superstable active state) and $J_{c-}$ (superstable inactive state), respectively. Using the continuum limit as in the preceding section, we find the following conditions:

- Superstable active state: $l_-(u) = l'_-(u) = 0$, with $l_-(u) = \epsilon y(u)e^{Ju/2} - z(u) - \frac{k_2}{k_3}\left[u + y - \epsilon z(u)e^{Ju/2}\right]$.
- Superstable inactive state: $l_+(u) = l'_+(u) = 0$, with $l_+(u) = y(u)e^{Ju} - \epsilon[u + y(u)]$.

Here, $z(u) = 1 - x(u) - y(u)$ with $x(u)$ and $y(u)$ given in Eq. (S5). Taking $k_3 \gg 1$, these equations are solved numerically for $J$ and $u$ to determine the phase boundaries $J_{c\pm}$ in Fig. 5D of the main text. The same calculation for various finite $k_3$ is shown in Fig. S2C. The location and order of the super-stability critical thresholds $J_{c\pm}$ changes with $k_3$ but the qualitative dependence on dissipation is maintained: the switchable region $J \in (J_c, \min(J_{c,\pm}))$ always expands with increasing dissipation $\Delta G$.

### 3. *Exact solution for $k_3 \gg 1$*

The effective potential underlying the mean-field dynamics can be obtained exactly under a separation of timescales $k_3 \gg 1$ (with $k_{-3}/k_3 = \epsilon$ fixed). In this limit, the system is in fast equilibrium in the $N_{-1}$ direction:

$$\frac{P(N_1, N_{-1}+1)}{P(N_1, N_{-1})} = \frac{N_0 k_3}{(N_{-1}+1)k_{-3}\exp\left(\frac{J(N_1-N_{-1})}{2(N-1)}\right)} = \epsilon^{-1}\frac{N_0}{N_{-1}+1}\exp\left(-\frac{J(N_1-N_{-1})}{2(N-1)}\right). \tag{S9}$$

In the continuum limit ($N \gg 1$), this implies fast equilibrium in the $y$ direction:

$$f_y \equiv \frac{1}{N}\frac{\partial \ln P(x,y)}{\partial y} = \ln\frac{1-x-y}{\epsilon y} - J(x-y)/2 + O(N^{-1}) = 0. \tag{S10}$$

Therefore, the probability distribution $P(x, y)$ is sharply peaked along the manifold $f_y = 0$ (with a width that vanishes with $N$). Along this manifold, the force along the $x$ direction is given by

$$f_x \equiv \frac{1}{N}\frac{\partial \ln P(x,y)}{\partial x}\bigg|_{f_y=0} = \ln\frac{y}{x} + J(x-y) + \ln\frac{k_1+\epsilon^2 k_2}{k_2+\epsilon k_1} + O(N^{-1}). \tag{S11}$$

As in the preceding sections, it is convenient to introduce the coordinate $u = x - y$, which explicitly solves $f_y = 0$:

$$f_y = 0 \Leftrightarrow x = \frac{u\epsilon e^{\frac{Ju}{2}} + u + 1}{\epsilon e^{\frac{Ju}{2}} + 2}. \tag{S12}$$

The force in the $u$ direction is

$$f_u = f_x\frac{\partial x}{\partial u} = \frac{\partial x}{\partial u}\cdot\left(\ln\left(1-\frac{u}{x}\right) + Ju + \ln\frac{k_1+\epsilon^2 k_2}{k_2+\epsilon k_1}\right), \tag{S13}$$

with $x(u)$ given by Eq. S12. The effective free energy landscape is $F(u) = -\int f_u\,\mathrm{d}u$.

In the two-state switching regime, $F(u)$ has two minima ($F'(u_{\pm 1}) = 0$, $F''(u_{\pm 1}) > 0$) which correspond to the active and inactive states, respectively. The free energy difference between these two states is

$$\frac{\Delta F}{N} = \frac{F(u_1) - F(u_{-1})}{N} = -\int_{u_{-1}}^{u_1} f_u\,\mathrm{d}u = \left[\log\frac{2+\epsilon}{2+\epsilon e^{\frac{Ju}{2}}} + \frac{1}{4}Ju(u+2) + \log(1-u)\right]_{u_{-1}}^{u_1}, \tag{S14}$$

where $u_{\pm 1}$ satisfy $f_u(u_{\pm 1}) = 0$, or equivalently $\ln\left(1-\frac{u}{x}\right) + Ju + \ln\frac{k_1+\epsilon^2 k_2}{k_2+\epsilon k_1} = 0$.

The two states are balanced (i.e. equal free energy and average dwell time) when $\Delta F = 0$. This is achieved when $\ln\frac{k_1+\epsilon^2 k_2}{k_2+\epsilon k_1} = 1$, or equivalently

$$k_1 = k_2(1+\epsilon). \tag{S15}$$

In this limit, the fixed points are determined by $\ln\left(1-\frac{u}{x}\right)+Ju=0$, which leads to three fixed points: an unstable fixed point $u_0=0$ corresponding to the free energy maximum, and a pair of stable fixed points $u_1=-u_{-1}$ corresponding to the free energy minima. Solving $f_u(u_{\pm 1})=0$ for $\epsilon$ gives

$$\epsilon=\frac{2\sinh\left(\frac{Ju}{2}\right)}{u}-2\cosh\left(\frac{Ju}{2}\right),\quad u=u_{\pm 1}, \tag{S16}$$

which simplifies the free energy difference to

$$\frac{\Delta F}{N}=\frac{F(u_1)-F(u_{-1})}{N}=\left[\frac{Ju^2}{4}+\log\frac{u-u\cosh\frac{Ju}{2}+\sinh\frac{Ju}{2}}{\sinh\frac{Ju}{2}}\right]_{u_{-1}}^{u_1}=0. \tag{S17}$$

Hence, the two states are indeed balanced. The critical coupling is determined by the stability of the $u_0=0$ fixed point:

$$\left.\frac{\partial f_u}{\partial u}\right|_{u=0}>0\Rightarrow J>J_c=2+\epsilon. \tag{S18}$$

Hence, the critical coupling $J_c=2+\epsilon=2+e^{-\Delta G/3}$ decreases monotonically from $J_c=3$ in the equilibrium limit to $J_c=2$ in the irreversible (infinite dissipation) limit. These two limits are consistent with the analytical results above. The linear relation between $J_c$ and $\epsilon$ is consistent with numerical results in Fig. S2A (solid black line) and near-equilibrium and large-dissipation expansions, Eqs. (S7) and (S8).

### 4. *Susceptibility scaling for $k_3 \gg 1$*

Using the exact solution from the preceding section, the steady-state distribution is $P(u)=e^{-F(u)}/Z$, where $Z=\int e^{-F(u)}\,du$ is the partition function. Since $F(u)\propto N$, for $N\gg 1$ this distribution is concentrated at points with zero-force $f_u(u)=0$. The average state is $\langle u\rangle=\int u\,P(u)\,du$ with susceptibility $\chi=-\left.\partial\langle u\rangle/\partial\Delta E_B\right|_{\Delta E_B=0}$. The barrier shift deforms the effective free energy $F(u)$ by scaling the forward and backward phosphorylation rate $k_{\pm 1}=k^0_{\pm 1}e^{\Delta E_B}$. Depending on the coupling strength, we have two possibilities:

- Disordered Phase ($J<J_c$). The distribution is tightly peaked at $u=0$ and the average $\langle u\rangle\approx 0$. To compute the susceptibility, we set Eq. (S13) to 0, differentiate with respect to $\Delta E_B$, and set $\Delta E_B=u=0$. The result is,

$$\chi=-\left.\frac{\partial\langle u\rangle}{\partial\Delta E_B}\right|_{u=0}=\frac{1-\epsilon^2}{(2+\epsilon-J)(1+\epsilon+\epsilon^2)} \tag{S19}$$

- Cooperative Phase ($J>J_c$). The distribution is tightly peaked at $u=u_{\pm 1}$, where $f_u(u_{\pm 1})=0$. The average state is then approximately,

$$\langle u\rangle=\frac{u_1+u_{-1}e^{\Delta F}}{1+e^{\Delta F}}=u_1\frac{1-e^{\Delta F}}{1+e^{\Delta F}}=-u_1\tanh\frac{\Delta F}{2}, \tag{S20}$$

where we have used $u_{-1}=-u_1$ (note, however, $\frac{\partial u_1}{\partial\Delta E_B}\neq\frac{\partial u_{-1}}{\partial\Delta E_B}$). The corresponding susceptibility has two contributions:

$$\chi=\frac{u_1}{2}\frac{\partial\Delta F}{\partial\Delta E_B}-\frac{1}{2}\left(\frac{\partial u_1}{\partial\Delta E_B}+\frac{\partial u_{-1}}{\partial\Delta E_B}\right)\equiv\chi_F+\chi_u \tag{S21}$$

Again these are readily computed using Eqs. (S13) and (S17) in the preceding sections. The final result is

$$\chi_F\equiv\frac{u_1}{2}\frac{\partial\Delta F}{\partial\Delta E_B}=N\cdot\frac{u(1-\epsilon)(\epsilon+1)\left(2u\left(\epsilon^2+2\right)e^{\frac{Ju}{2}}+(3u-1)\epsilon e^{Ju}+3u\epsilon+\epsilon\right)}{2\left(\epsilon^2+\epsilon+1\right)\left(2e^{\frac{Ju}{2}}+\epsilon\right)\left(\epsilon e^{\frac{Ju}{2}}+2\right)}, \tag{S22}$$

$$\chi_u\equiv-\frac{1}{2}\left(\frac{\partial u_1}{\partial\Delta E_B}+\frac{\partial u_{-1}}{\partial\Delta E_B}\right)=\frac{2(1-u)\left(1-\epsilon^2\right)\left(u\epsilon e^{\frac{Ju}{2}}+u+1\right)}{\left(\epsilon^2+\epsilon+1\right)\left(2J\left(u^2-1\right)+\epsilon e^{\frac{Ju}{2}}(J(u-1)u+2)+4\right)}, \tag{S23}$$

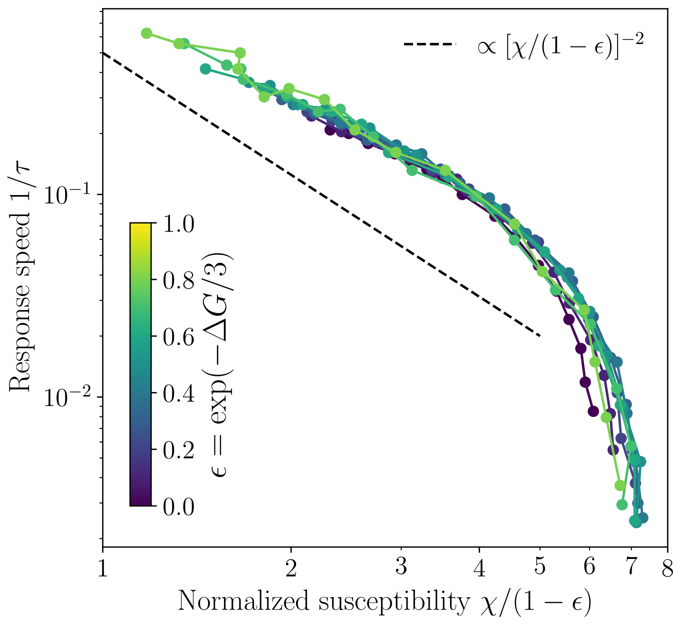


FIG. S3. Scaling collapse of the speed-sensitivity trade-off. Data are identical to Fig. 4B in the main text, with the susceptibility $\chi$ normalized by a dissipation-dependent factor $(1-\epsilon)$, which collapses the curves up to a weak additional $\epsilon$-dependence. For subcritical coupling ($J < J_c$) we see a power-law relation $\tau^{-1} \sim [(1-\epsilon)/\chi A(\epsilon)]^{\zeta}$, with exponent $\zeta$ slightly less than 2 (black dashed line). For supercritical coupling ($J > J_c$), the speed is exponentially suppressed by the free energy barrier, $\ln \tau^{-1} \sim -\chi/(1-\epsilon)C(\epsilon)$.

where on the right-hand side of these equations $u$ stands for $u_1 = -u_{-1}$. For large $N$, $\chi_F$ dominates except near $J_c$, where $\chi_u$ dominates. Note that for a finite $N$, rather than diverging at the critical point ($J \to J_c = 2 + \epsilon$), $\chi_u$ has a maximum of order $O(N^{1/2})$, which is small compared to the susceptibility, $\chi_F \sim O(N)$, within the cooperative phase. Thus for finite systems, the susceptibility is a smoothly increasing function of $J$. This contrasts with the usual peaked susceptibility in the Ising model because we are studying the susceptibility of the average activity $\langle a \rangle$ on a timescale that includes switching events that, for example, flip the entire system from active to inactive.

The susceptibility expressions above, Eqs. (S19)-(S23), each contain an overall factor of $(1-\epsilon)$. Scaling the measured susceptibility from lattice simulations by $(1-\epsilon)$, we find that the speed-sensitivity trade-off (main text Fig. 4B), approximately collapses onto a single curve (Fig. S3). The shape of this curve can be understood by again considering the two phases:

- Disordered Phase. The response speed is determined by the curvature near the minimum of the free energy. In the mean-field theory, we have $\tau^{-1} \sim F''(0) \sim (J_c - J) \sim (1-\epsilon)/\chi A(\epsilon)$. In the lattice model we expect similar scaling with a modified exponent, $\tau^{-1} \sim [(1-\epsilon)/\chi A(\epsilon)]^{\zeta}$. In terms of traditional critical exponents $\zeta = \nu z/\gamma$, where $\nu$, $\gamma$ are the exponents for the correlation length and susceptibility and $z$ is the dynamic exponent. In the disordered phase (with fast response, low susceptibility), we find $\zeta \lesssim 2$ (Fig. S3), though the power law is maintained over less than an order of magnitude.

- Cooperative Phase. Here the response speed is exponentially suppressed by the free energy barrier, $\ln \tau^{-1} \sim -\Delta F \sim -(J - J_c)B(\epsilon) \sim -\chi/(1-\epsilon)C(\epsilon)$. Indeed in Fig. S3, we see an exponential fall-off in the speed-susceptibility scaling collapse in the cooperative phase (with slow response, large susceptibility).

Since the speed-susceptibility curves collapse nicely after scaling by $(1-\epsilon)$, the functions $A(\epsilon)$, $B(\epsilon)$, and $C(\epsilon)$ in the analysis above should only weakly depend on $\epsilon$.

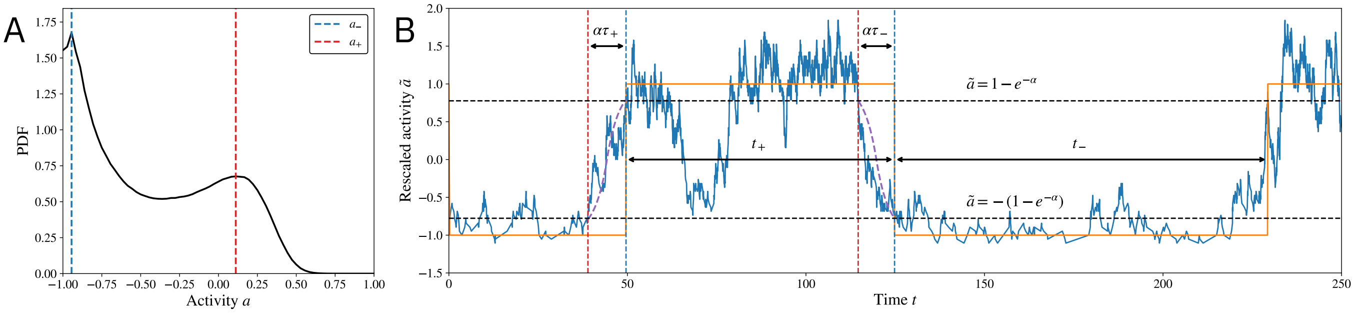


FIG. S4. Illustration of the numerical scheme for determining the dwell time and switching time. (A) Sample histogram of the lattice mean activity, where the peaks define the two states $a_\pm$. (B) Sample trajectory (blue line) of the rescaled activity $\tilde{a} = \frac{2a-(a_+ + a_-)}{a_+ - a_-}$, which exhibits two state-switching between $\tilde{a} = \pm 1$ (orange line). The horizontal blacked dashed lines indicate thresholds for switching $\pm(1 - e^{-\alpha})$ with $\alpha = 1.5$. The vertical dashed lines indicate the start (red) and end (blue) of two switching events, the duration of which is $\alpha\tau_\pm$ with $\tau_\pm$ defined as the switching times following ref. [2, 3]. The dwell times $t_\pm$ are defined as the duration between switching events.

### B. Effective Hill coefficient with respect to ligand concentration

The sensitivity of the kinase activity in response to ligand concentration is given by

$$H \equiv 2 \frac{\mathrm{d} \log \langle \tilde{a} \rangle}{\mathrm{d} \log [L]} \bigg|_{\langle \tilde{a} \rangle = 1/2} = \left( - \frac{\partial \langle \tilde{a} \rangle}{\partial \Delta E_B} \right) \left( - \frac{1}{\langle \tilde{a} \rangle} \frac{\partial \Delta E_B}{\partial \log [L]} \right) = \frac{4\chi}{a_{\max} - a_{\min}} \left( - \frac{\partial \Delta E_B}{\partial \log [L]} \right). \tag{S24}$$

where $\langle \tilde{a} \rangle = \frac{a_{\max} - \langle a \rangle}{a_{\max} - a_{\min}}$ is the normalized kinase activity, $a_{\min} = \langle a \rangle \big|_{[L] \to \infty}$ and $a_{\max} = \langle a \rangle \big|_{[L] \to 0}$ are respectively the minimum and maximum kinase activities, and $\chi = -\partial \langle a \rangle / \partial \Delta E_B \big|_{\Delta E_B = 0}$ is the susceptibility, as in the main text. The factor 2 is introduced so that $H$ gives the exact Hill coefficient $H = H_0$ if $\langle \tilde{a} \rangle$ is given by a Hill function $\frac{[L]^{H_0}}{[L]^{H_0} + K_H^{H_0}}$.

As discussed in the main text, the effective barrier shift is $\Delta E_B = \alpha n (m - m_0) + n \ln \left( \frac{1 + [L]/K_i}{1 + [L]/K_a} \right)$ if the relation between receptor conformation and occupancy is described by the MWC model. The sensitivity is then

$$H_{\mathrm{MWC}} = \frac{4n\chi}{A} \frac{(K_a - K_i)[L]_0}{(K_a + [L]_0)(K_i + [L]_0)}, \tag{S25}$$

where $A = a_{\max} - a_{\min}$ is the total range of activity response and where $[L]_0$ is the half-maximum concentration $\langle \tilde{a} \rangle ([L]_0) = 1/2$. Note that the sensitivity $S$ scales linearly with both the MWC cluster size $n$ and the lattice susceptibility $\chi$. The last factor is:

$$\frac{(K_a - K_i)[L]_0}{(K_a + [L]_0)(K_i + [L]_0)} \le \frac{(K_a - K_i)}{\left(\sqrt{K_a} + \sqrt{K_i}\right)^2} < 1. \tag{S26}$$

Therefore, the maximum sensitivity is

$$H_{\mathrm{MWC,\ max}} = 4A^{-1} n \chi. \tag{S27}$$

The maximum is reached when $[L]_0 = \sqrt{K_i K_a}$ and is approximately attained as long as $K_i \ll [L]_0 \ll K_a$.

## II. SUPPLEMENTAL NUMERICAL RESULTS

### A. Numerical scheme for determining the dwell time and switching time

We use the standard Gillespie algorithm [1] to simulate the dynamics of our nonequilibrium lattice model. The system is initialized at a random configuration and run for $10^6$ time steps to reach steady state, after which a

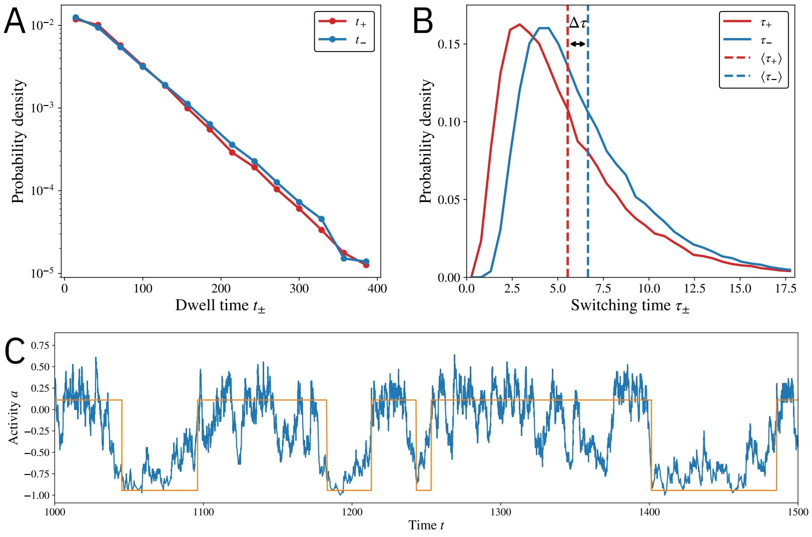


FIG. S5. Asymmetric two-state switching in the hexagonal lattice. (A–B) The distribution of dwell time (A) and switching time (B). (C) Sample trajectory of the activity $a$ (blue), which is segmented into active and inactive states (orange). Parameters: $J = 0.75$, $k_2 = 1$, $k_3 = 0.5$, $\epsilon = 0$. Lattice size $N = 36$. The rate $k_1 = 1.497$ is chosen to achieve (approximately) equal dwell times in the active and inactive states.

long trajectory is generated to evaluate the switching statistics. In the two-state switching regime, the activity $a(t)$ exhibits bimodal distribution (Fig. S4A), where the position of the peaks gives the activity of the two states $a_\pm$. It is convenient to rescale the activity by $\tilde{a}(t) = \frac{2a(t)-(a_+ + a_-)}{a_+ - a_-}$ so that activity switches between $\tilde{a} = \pm 1$ (Fig. S4B). We define switching events by crossing the threshold $(1 - e^{-\alpha})$ from below (switching to the active state) or crossing the threshold $-(1 - e^{-\alpha})$ from above (switching to the inactive state). The dwell time $t_\pm$ is the duration between switching events. Following the switching time definition in Refs. [2, 3], we assume that the switching trajectory follows the functional form:

$$\tilde{a}(t - t_0) = \pm \frac{t - t_0}{|t - t_0|}\left(1 - e^{-2|t-t_0|/\tau_\pm}\right), \tag{S28}$$

where $\tau_\pm$ is the switching time and the sign $\pm$ depends on the direction of switching (+ for switching up and − for switching down). Under this assumption, the time for crossing the thresholds (red and blue dashed lines in Fig. S4B) is $t_{1,2} = t_0 \pm \frac{\alpha\tau_\pm}{2}$, which gives the switching time by $\tau_\pm = \frac{t_2 - t_1}{\alpha}$. We take a moderate threshold $\alpha = 1.5$ to avoid either missing switching events or finding spurious switching events.

## B. Two-state switching in other lattice structures

The two-state switching behavior analyzed in the main text does not rely on the specific lattice structure. To illustrate this, we simulate our nonequilibrium lattice model on a hexagonal lattice, which better captures the connectivity structure of the chemoreceptor cluster in *E. coli* [4]. Above the critical coupling, the system exhibits two-state switching (Fig. S5C) with exponentially distributed dwell times (Fig. S5A) and asymmetric, right skewed switching times (Fig. S5B), which are qualitatively identical to the square lattice (main text Fig. 1).

## C. Scaling of asymmetric switching statistics with lattice size

In the main text, we have focused on a fixed lattice size $N = 36$ to demonstrate the roles of near-critical coupling $J$ and energy dissipation $\Delta G$ in producing asymmetric switching dynamics and enhancing chemotaxis signaling. Increasing lattice size $N$ does not change the asymmetric switching behavior qualitatively. Fig. S6 shows the switching/dwell time ratio and switching time asymmetry for a larger lattice ($N = 100$). Consistent with main text Fig. 2 ($N = 36$), switching time asymmetry is maximized in the regime of high dissipation $\Delta G$ (small $\epsilon = e^{-\Delta G/3}$) and near-critical

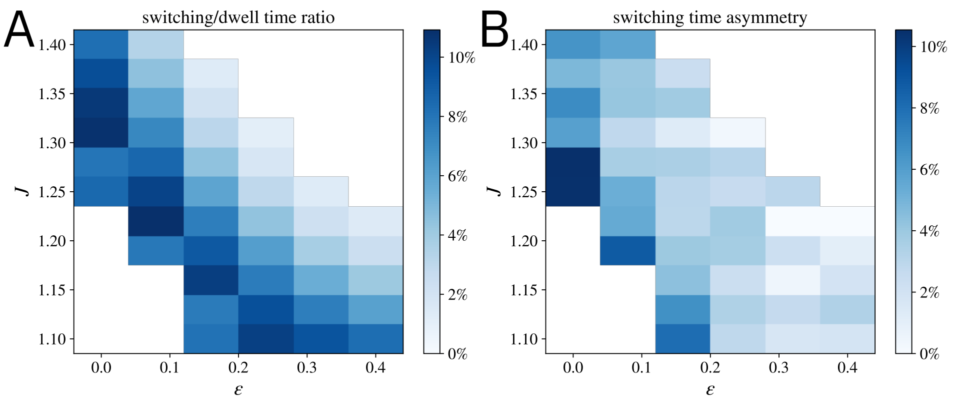


FIG. S6. Heatmaps of switching/dwell time ratio (A) and switching time asymmetry (B) as functions of $J$ and $\epsilon = e^{-\Delta G/3}$. Parameter: $k_3 = 0.1$. Lattice size: $N = 100$. Only points with switching/dwell time ratio $\langle \tau_\pm \rangle \,/\, \langle t_\pm \rangle > 1\%$ are plotted in order to ensure sufficient statistics.

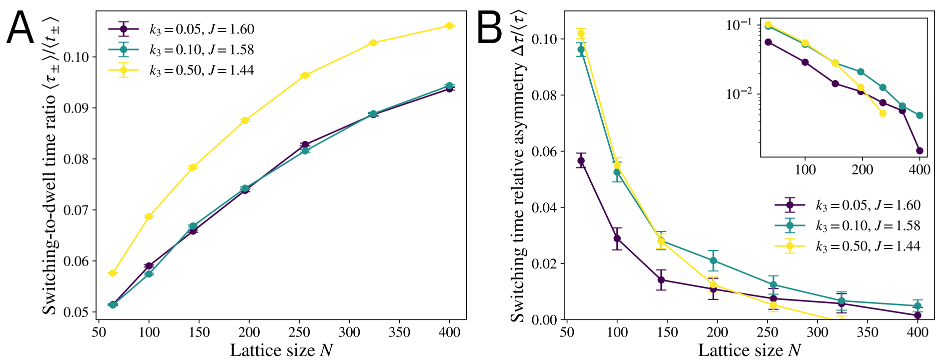


FIG. S7. Scaling of switching/dwell time ratio (A) and switching time asymmetry (B) with the lattice $N = L \times L$ for different values of $k_3$ and $J$ (see legends). Inset of (B) is in log-log scale. All simulations are done in the infinite dissipation limit $\epsilon = 0$.

coupling (which is represented by a large switching-to-dwell time ratio). These results indicate that energy dissipation and proximity to criticality are necessary for the observed asymmetric switching behavior, regardless of the lattice size.

To more systematically investigate how lattice size affects switching time asymmetry, we ran Gillespie simulations for increasing lattice sizes $N$ with $J$ and $k_3$ fixed and in the infinite dissipation limit ($\epsilon \to 0$). As shown in Fig. S7A, for fixed coupling $J$, the switching-to-dwell time ratio increases slowly with the lattice size $N$. Its value is comparable to experimental measurements of 0.08-0.12. The increase is due to the critical coupling $J_c$ increasing with lattice size $N$. This indicates that while proximity to criticality is essential for observing switching, the coupling strength $J$ can still vary within a reasonably relaxed range in order to explain the experimentally observed switching dynamics. On the other hand, the switching time asymmetry generally decreases with lattice size $N$ (Fig. S7B), but the rate of decrease is dependent on parameters such as $k_3$ and $J$, as well as details of the kinase reaction cycle which is assumed to be a simple three-state cycle in this work. As discussed in the main text (sections *"Chemoreceptor array operates near a highly nonequilibrium critical point"* and *"Discussion"*), incorporating a more detailed description of the reaction cycle may lead to larger asymmetry that also decays more slowly as $N$ increases. This is further supported by results in the mean-field model– -see the following section and Figs. S8 and S9.

### D. Finite-size scaling of asymmetric switching statistics in the mean-field model

To further investigate the finite-size scaling of two-state switching dynamics, we numerically compute first passage statistics directly from the mean-field master equation defined in Eqs. (S1) and (S2). The numerical calculation of dwell and switching times is carried out as follows. First, we determine the steady-state distribution of the master equation (i.e., the null vector of the transition matrix) and project this distribution onto the activity axis $a = (N_1 - N_{-1})/N$. The active and inactive states are defined identically to the lattice model (see SI Section II A and

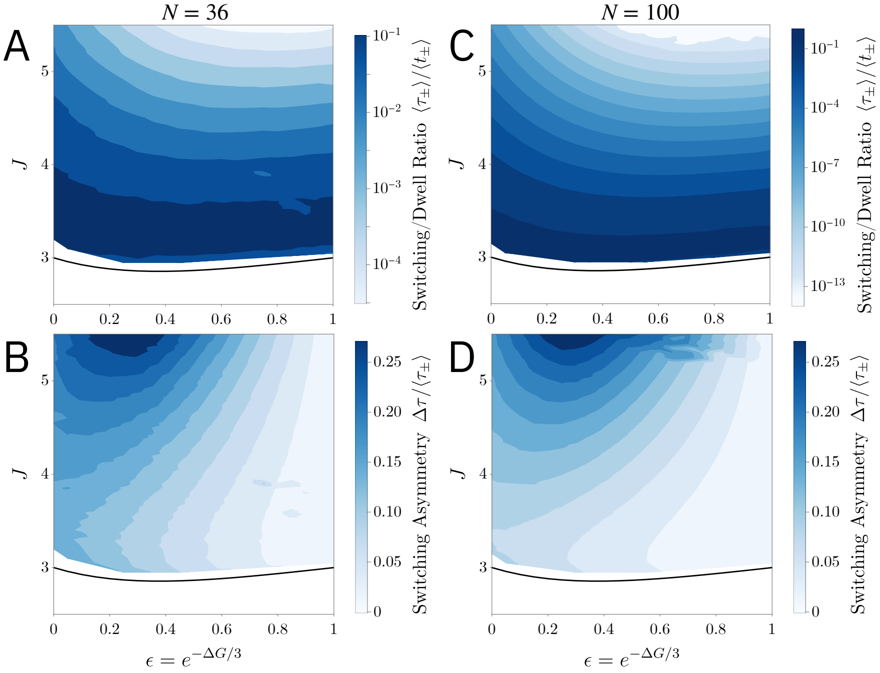


FIG. S8. Switching-to-dwell-time ratio (A and C) and switching time asymmetry (B and D) in the mean-field model for system sizes $N = 36$ (A-B) and $N = 100$ (C-D). Dwell times grow exponentially with $J$ and system size. Switching asymmetry decreases moderately with system size for a given $(J, \epsilon)$. Behavior is qualitatively similar to lattice simulations (c.f. main text Fig. 2B and D and Fig. S6). In each panel, the black line shows the $N \to \infty$ critical boundary $J_c(\epsilon)$ computed using Eq. (S6). All calculations use $k_3 = 0.5$.

Fig. S4): we extract peaks $a_\pm$ from the activity distribution $P(a)$ and use relative thresholds $\pm(1 - e^{-\alpha})$ to define the collection of microstates that make up the active and inactive states. In particular, the active state is defined by $a > \frac{a_+ + a_-}{2} + (1 - e^{-\alpha})\frac{a_+ - a_-}{2}$, and the inactive state is $a < \frac{a_+ + a_-}{2} - (1 - e^{-\alpha})\frac{a_+ - a_-}{2}$.

Given the collection of active and inactive states, the dwell and switching times can be exactly computed using the backward master equation with appropriate boundary conditions, following standard approaches in transition-state theory [5, 6]. Specifically, for dwell times we compute the average first-passage time to the target states with initial conditions averaged over the steady state distribution within the source states. For switching times, both active and inactive states are made absorbing and we compute the conditioned first-passage time to the target states. Here, initial conditions are the states neighboring the source states, weighted by their likelihood of occurrence at steady state. In the results described below, for each choice of parameters $(N, J, \Delta G, k_3)$, we vary $k_1$ to balance the forward and backward dwell times so that the system spends the same amount of time in active and inactive states, as is done in the lattice Gillespie simulations.

This mean-field calculation allows us to probe the behavior of switching dynamics beyond what is feasible in Gillespie simulations of the lattice model since it gives us exact switching time statistics that are not limited by directly observing rare events. We computed switching time phase portraits in the $(\epsilon, J)$-plane (analogous to main text Fig. 2B and D and Fig. S6) over a broad range of coupling strengths for $N = 36$ and $N = 100$, see Fig. S8. Consistent with the lattice simulations, we find that the switching time is always asymmetric for $\epsilon < 1$ $(\Delta G > 0)$, with moderate decreases as $N$ grows. In contrast to the lattice results, the finite-size scaling of the critical coupling $J_c$ is relatively weak. Thus for fixed coupling, dwell times grow considerably. Nonetheless, there is a reasonable range of couplings for which the switching-to-dwell ratio is comparable to the experimentally observed timescales. Interestingly, the mean-field model exhibits increasing switching asymmetry for large coupling strengths, though in this regime switching events are exceedingly rare and difficult to observe in direct kinetic simulations. We also see non-monotonicity with $J$: the asymmetry increases moderately as we approach the critical point from above, similar to the behavior observed in lattices.

We additionally compute the scaling of the switching time asymmetry while varying coupling strength $J$ to fix the switching-to-dwell-time ratio in the experimentally measured value $\langle\tau_\pm\rangle/\langle t_\pm\rangle = 0.08$. Fig. S9 shows the resulting switching time asymmetry $\Delta\tau/\langle\tau_\pm\rangle$ and coupling strength $J/J_c - 1$ (relative to the critical coupling) and as a function of system size. Again we consistently find non-zero switching asymmetry that moderately decreases as the system size grows. As demonstrated by the Fig. S9 insets the scaling is power-law; we find exponents roughly in the range

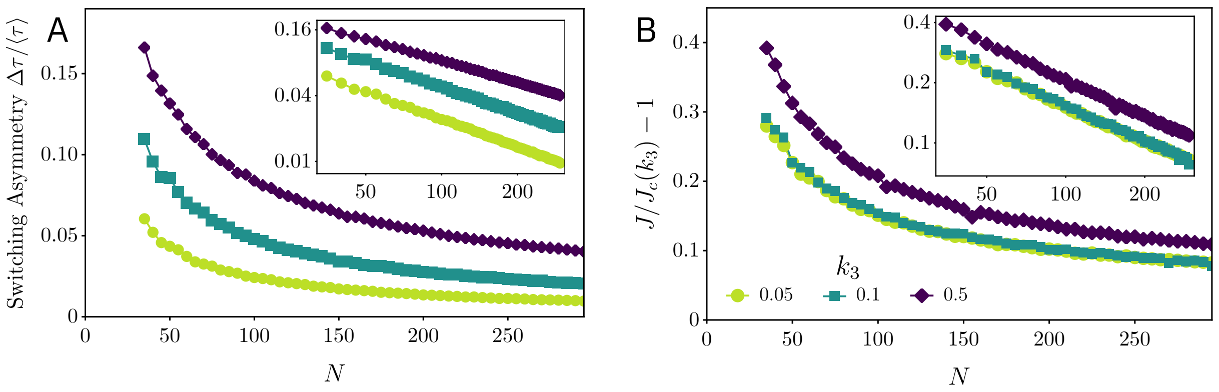


FIG. S9. Finite-size scaling of mean-field switching time asymmetry (A) and the relative distance to the critical point (B) with $J$ tuned to fix the switching-to-dwell-time ratio to the experimentally observed value, $\langle\tau_\pm\rangle/\langle t_\pm\rangle = 0.08$. All calculations are done in the infinite dissipation limit $\epsilon = 0$. Each panel shows results for $k_3 = 0.05$ (circles), $k_3 = 0.1$ (squares), and $k_3 = 0.5$ (diamonds). Insets show the same data on log-log scale, indicating that the scaling is roughly power-law with exponent and amplitude dependent on $k_3$. Fixing the switching-to-dwell-time ratio only requires tuning within $\sim 10\%$ of the critical coupling.

$0.5-1.0$ indicating a relatively slow decay of the switching asymmetry with system size. The power-law scaling is also observed in lattice Gillespie simulations (Fig. S7B inset). The result in Fig. S9B indicates that even for relatively large systems (up to $N = 300$), the coupling strength only needs to be tuned within $\sim 10\%$ of $J_c$ achieve the experimentally observed switching-to-dwell-time ratio. Finally, both the overall magnitude and finite-size scaling of the switching time asymmetry and coupling strength depend on the $k_3$, i.e. the details of the underlying kinetics. This indicates that a more complicated and biologically realistic kinetic cycle could maintain considerable switching time asymmetries even in large systems (see section *Disussion* in the main text).

### E. Response functions

In Fig. 4B of the main text, we demonstrated a speed-sensitivity trade-off due to varying the coupling strength $J$ for a small signal $\Delta E_B = -0.1$. Here, we show that this trade-off cannot be completely removed even by going to the nonlinear (large signal) regime. Fig. S10A shows the trade-off curves between response speed (quantified by the inverse of response time $\tau^{-1}$) and amplitude (quantified by the change in activity $\Delta\langle a\rangle$) for a large signal $\Delta E_B = -0.5$. Increasing coupling $J$ increases the amplitude at the cost of speed, which is more explicitly shown in Fig. S10B. Increasing the dissipation $\Delta G$ improves both response speed and amplitude (Fig. S10C), thus shifting the trade-off curves in Fig. S10A to the upper right.

Fig. 4C of the main text shows a speed-sensitivity trade-off due to varying the dissipation $\Delta G$, which is in general removed when the signal is sufficiently large (Fig. 5A of the main text). Another potential way of removing the trade-off is to reduce $k_3$. At a small $k_3$, speed-sensitivity trade-off still exists when varying the coupling $J$ (Fig. S11A). However, increasing dissipation $\Delta G$ enhances both speed and sensitivity (Fig. S11B). Thus, the trade-off in Fig. 4C of the main text is a worst-case scenario when $k_{\pm 3}$ is large (relative to the unit of time set by $k_2$).

In the main text, we mentioned that the response functions of other order parameters (e.g. $N_1$, the number of core units in the "active state") behave similarly to the response of the lattice activity $\langle a\rangle$. Figs. S12 and S13 show the response, susceptibility, and trade-offs for $\langle N_1/N\rangle$. Comparing to the response of $\langle a\rangle$ (main text, Figs. 4 and 5), we see that the $N_1$ has nearly identical response properties, but with a slightly smaller amplitude. This indicates that total response of $\langle a\rangle = (N_1 - N_{-1})/N$ to an increase in $\Delta E_B$ is approximately evenly split between decreasing $N_1$ and increasing $N_{-1}$.

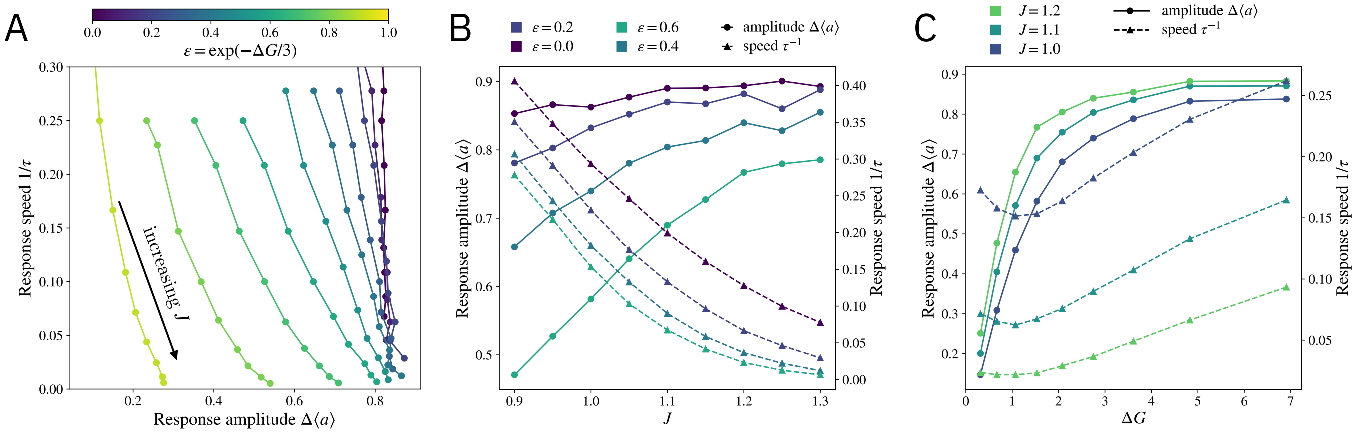


FIG. S10. Response speed (quantified by the inverse of response time $\tau^{-1}$) and amplitude (quantified by the change in activity $\Delta\langle a\rangle$) for a large input signal, $\Delta E_B = -0.5$. (A) Response speed versus amplitude. Each line represents a fixed dissipation level $\Delta G$ with different coupling $J$. (B) Response speed (dashed lines) and amplitude (solid lines) for fixed dissipation $\Delta G$ as a function of coupling strength $J$. (C) Response speed (dashed lines) and amplitude (solid lines) for fixed coupling $J$ and different levels of dissipation $\Delta G$. Parameters are identical to Fig. 4 of the main text: $k_3 = 2.5$, lattice size $N = 6 \times 6$.

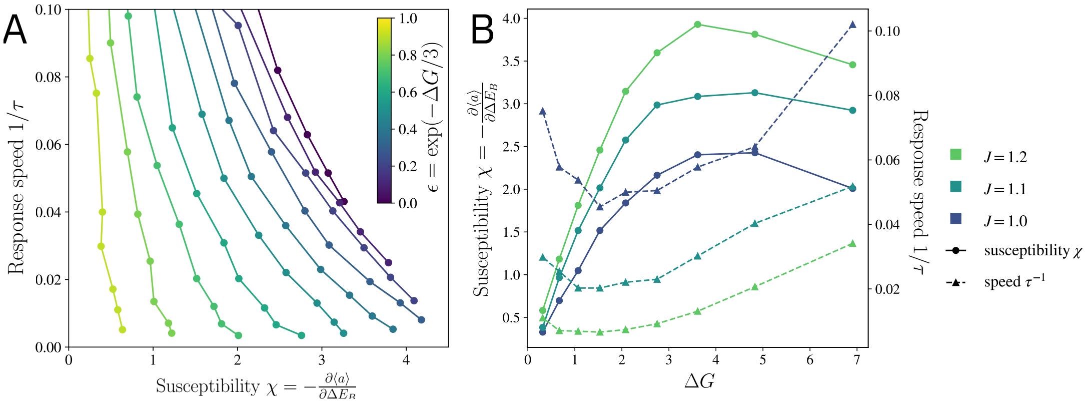


FIG. S11. Speed-sensitivity trade-off due to $\Delta G$ may be relieved by reducing $k_3$. (A) Response speed versus amplitude. Each line represents a fixed dissipation level $\Delta G$ with different coupling $J$. (B) Response speed (dashed lines) and amplitude (solid lines) for fixed coupling $J$ and different levels of dissipation $\Delta G$. Parameters: $k_3 = 0.5$, lattice size $N = 6 \times 6$.

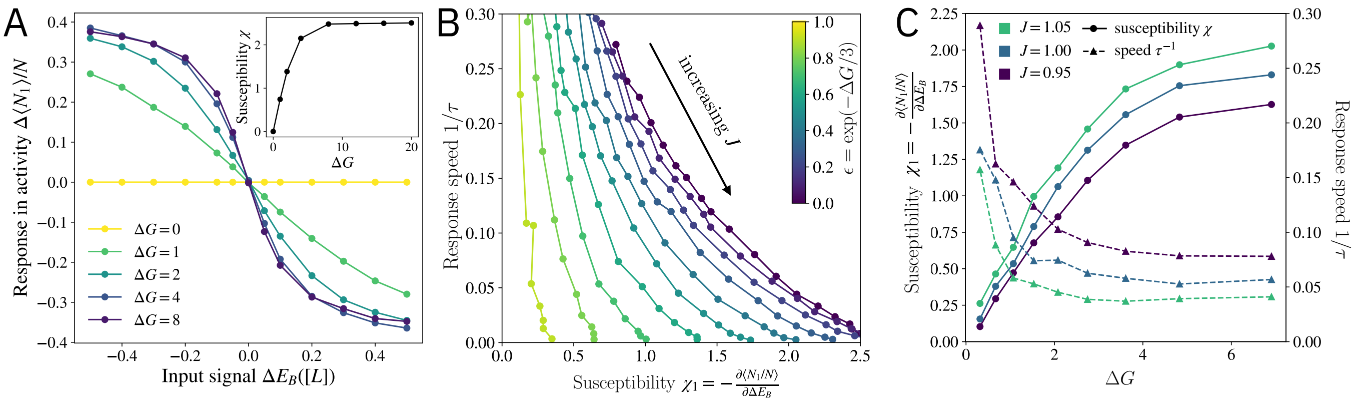


FIG. S12. Response function for the fraction, $N_1/N$, of core units in the active state. (A) The change in activity $\langle N_1/N\rangle$ due to an external signal $\Delta E_B([L])$ for various dissipation levels $\Delta G$. The inset shows the susceptibility $\chi = -\left.\frac{\partial\langle N_1/N\rangle}{\partial \Delta E_B}\right|_{\Delta E_B=0}$. (B) Linear response speed $\tau^{-1}$ versus susceptibility $\chi$. Each line represents a fixed dissipation level $\Delta G$ (see inset legend) with different couplings $J$. Large dissipation improves the speed-amplitude trade-off. (C) At fixed coupling $J$ and in the linear regime ($\Delta E_B \ll 1$), increasing dissipation $\Delta G$ enhances susceptibility (solid lines) at the cost of response speed (dashed lines). For (B–C), susceptibility is computed by $\chi = -\frac{\Delta\langle N_1/N\rangle}{\Delta E_B}$ with a small applied field $\Delta E_B = -0.1$; $\tau$ is obtained by fitting the exponential relaxation of the activity $x(t) = x_\infty + \Delta x e^{-t/\tau}$, with $x(t) = \langle N_1/N\rangle$. We use $k_3 = 2.5$ in all panels. The shape of the response curves for $\langle N_1/N\rangle$ is nearly identical to that of $\langle a\rangle$ (c.f. main text Fig. 4), despite smaller amplitudes.

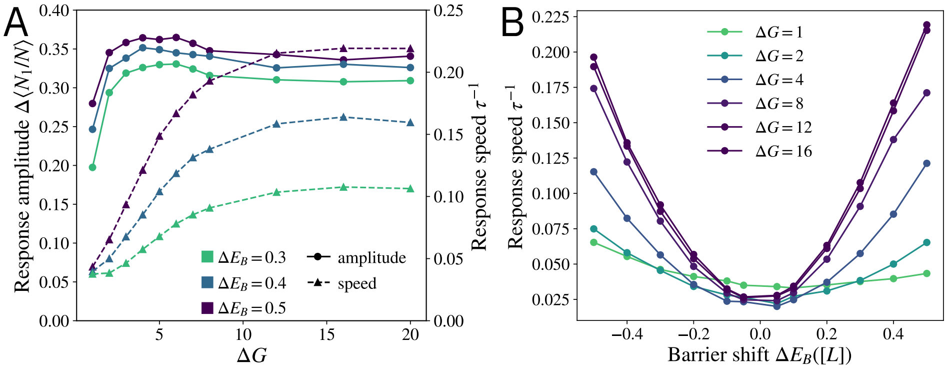


FIG. S13. Nonlinear response for the fraction of active core units $\langle N_1/N\rangle$. (A) Response amplitude $\Delta\langle N_1/N\rangle$ (solid lines) and response speed $\tau^{-1}$ (dashed lines) as functions of dissipation $\Delta G$ at large external signals $\Delta E_B([L])$. (B) The response speed as a function of the barrier shift $\Delta E_B([L])$ for different dissipation levels. The shape of the response curves for $\langle N_1/N\rangle$ is nearly identical to that of $\langle a\rangle$ (c.f. main text Fig. 5).

## REFERENCES


[1] D. T. Gillespie, Exact stochastic simulation of coupled chemical reactions, J. Phys. Chem. **81**, 2340 (1977).

[2] J. M. Keegstra, F. Avgidis, Y. Mullah, J. S. Parkinson, and T. S. Shimizu, Near-critical tuning of cooperativity revealed by spontaneous switching in a protein signalling array, bioRxiv 10.1101/2022.12.04.518992 (2022).

[3] J. M. Keegstra, K. Kamino, F. Anquez, M. D. Lazova, T. Emonet, and T. S. Shimizu, Phenotypic diversity and temporal variability in a bacterial signaling network revealed by single-cell FRET, eLife **6**, e27455 (2017).

[4] J. S. Parkinson, G. L. Hazelbauer, and J. J. Falke, Signaling and sensory adaptation in Escherichia coli chemoreceptors: 2015 update, Trends in Microbiology **23**, 257 (2015).

[5] N. G. Van Kampen, *Stochastic processes in physics and chemistry*, Vol. 1 (Elsevier, 1992).

[6] S. Redner, *A Guide to First-Passage Processes* (Cambridge University Press, 2001).
